# Supplementary material for: Hide & Seek: Transformer Symmetries Obscure Sharpness & Riemannian Geometry Finds It
Source: arXiv:2505.05409 source file (2025-05-08)
Supplement: Supplementary file 1 [file attention.tex]

We now describe how the $\GL$ symmetry gives to rise to a quotient Riemannian manifold

$\gE \coloneqq \sR^{n \times h} \times \sR^{m \times h} \simeq \sR^{(n + m) h}$

In what follows we restrict our weight matrices to have full column rank.

\begin{assumption}[]
  The rank of $\mG, \mH$ corresponds to their number of columns, $\rank(\mG) = \rank(\mH) = h$.
\end{assumption}
This implies $h \le n,m$, which is usually satisfied in (multi-head) attention layers (\Cref{ex:self-attention}) for the default choices of $d_{\text{v}}, d_{\text{k}}$, as well as for LoRA (\Cref{ex:lora}).
In the following, we therefore restrict both $\mG, \mH$ to the set of fixed-rank matrices,
\begin{subequations}
  \begin{align}
    \overline{\gM}
    &\leftarrow
      \sR^{n \times h}_h
      \times
      \sR^{m \times h}_h
      \shortintertext{where}
      \sR^{n \times h}_k
    &\coloneq
      \left\{
      \mB \in \sR^{n \times h} \mid \rank(\mB)=k
      \right\}\,.
  \end{align}
\end{subequations}
We can represent a point $\bar{x} \in \overline{\gM}$ by a matrix tuple $(\mG, \mH) \in \sR^{n \times h}_h \times \sR^{m \times h}_h$. Its tangent space $\mathrm{T}_{\bar{x}}\overline{\gM}$ is
\begin{align}
  \mathrm{T}_x\overline{\gM}
  =
  \left\{ \eta \in \sR^{n \times h} \times \sR^{m \times h} \right\}
\end{align}
and a tangent vector $\eta \in \mathrm{T}_{\bar{x}}\overline{\gM}$ is represented by a matrix tuple $(\eta_{\mG}, \eta_{\mH}) \in \sR^{n \times h} \times \sR^{m \times h}$.

We endow $\overline{\gM}$ with the metric $\langle  \cdot, \cdot \rangle_{\bar{x}}: \mathrm{T}_{\bar{x}} \overline{\gM} \times \mathrm{T}_{\bar{x}} \overline{\gM} \to \sR$,
\begin{small}%
  \begin{align}%
    \langle \eta, \zeta \rangle_x
    =
    \Tr
    \left(
    ( \mG^{\top}\mG )^{-1}
    \eta_{\mG}^{\top} \zeta_{\mG}
    +
    ( \mH^{\top}\mH )^{-1}
    \eta_{\mG}^{\top} \zeta_{\mG}
    \right)\,,
  \end{align}%
\end{small}%
different from the Euclidean metric that simply flattens and concatenates the matrix tuples into vectors and takes their dot product, $\langle \eta, \zeta \rangle = \Tr \left( \eta_{\mG}^{\top} \zeta_{\mG} + \eta_{\mH}^{\top} \zeta_{\mH} \right)$. Importantly, this metric is invariant under the symmetries of the attention mechanism. Which means that it defines a valid metric on the quotient manifold \todomf{Insert reference to Absil/Boumal here}.

The quotient space's elements are equivalence classes of the symmetry-induced equivalence relationship on the total space.
For two elements $\bar{x}, \bar{x}' \in \overline{\gM}$ represented by the tuples $(\mG, \mH), (\mG', \mH')$ we have
\begin{align}
  x \sim x'
  \
  \Leftrightarrow
  \
  (\mG,\mH)
  % =
  % \psi(\mA, x')
  =
  (\mG'\mA^{-1}, \mH'\mA^\top)
\end{align}
for some $\mA \in \GL(h)$.
A point $[x]$ on the quotient space is the equivalence class
\begin{align}
  [x]
  =
  \left\{
  (\mG \mA^{-1}, \mH \mA^\top)
  \mid
  \mA \in \GL(h)
  \right\}
\end{align}
with \emph{natural projection} $\pi \colon \overline{\gM} \to \gM, x \mapsto [x]$.
We leave all of the details to Appendix~\ref{quotient-appendix}, but we can apply the general program of Section~\ref{sec:conceptual} to obtain formulas for the Riemannian gradient, and the Riemannian Hessian:
\begin{align*}
    \operatorname{grad} f(\mG, \mH)=\left(\nabla_{\mG} f(X) \mG^T \mG, \nabla_{\mH} f(X) \mH^T \mH\right)
\end{align*}
where,  $\nabla f(x) = \left(\nabla_{\mG} f(X), \nabla_{\mH} f(X)\right)$.

The horizontal space is the vertical space's orthogonal complement w.r.t.\,the metric $\langle \cdot, \cdot \rangle_x$.
Let's take a tangent vector $\xi \in \mathrm{T}_x \overline{\gM}$ and decompose it into $\xi = \xi^{\text{V}} + \xi^{\text{H}}$ where $\xi^{\text{V}}$ has the form of \Cref{eq:vertical-space}.
This immediately yields
\begin{equation}
  \mathrm{H}_x \overline{\gM}
  =
  \left\{(
    \xi_{\mG} + \mG \mLambda,
    \xi_{\mH} -\mH \mLambda^\top
    ) \mid \xi
    \in  \mathrm{T}_x \overline{\gM}
  \right\}
\end{equation}
To determine $\mLambda$, insert into the orthogonality equation $\langle \xi^{\text{V}}, \xi^{\text{H}} \rangle_x = 0$, which yields a Sylvester equation \fd{Double-check this expression and the abbreviations $\mA, \mB$.}
\begin{align}\label{equ:lyapunov-equation}
  \mA \mLambda + \mLambda \mA^{\top}  = \mB
\end{align}
with $\mA = \mG^\top \mG \mH^\top \mH$,
$\mB = \mG^\top \mG \mH^\top \xi_{\mH} - \xi_{\mG}^{\top} \mG \mH^\top \mH$.
With that, we can write down the projector onto the horizontal space:
\begin{align*}
   \mathrm{Proj}_x^{\text{H}}(\xi)
  = \xi^{\text{H}}
  = (\xi_{\mG} + \mG \mLambda, \xi_{\mH} -\mH \mLambda^\top)
\end{align*}
where $\mLambda$ is the solution of \Cref{equ:lyapunov-equation}.
