# Supplementary material for: Hide & Seek: Transformer Symmetries Obscure Sharpness & Riemannian Geometry Finds It
Source: arXiv:2505.05409 source file (2025-05-08)
Supplement: Supplementary file 2 [file shallow_linear_net_matrix_weights.tex]

Here, we consider a generalized form of the shallow linear network from \Cref{sec:shallow-linear-net-scalar-weights} with matrix-valued weights.
We perform numerical investigations for the matrix case whose Riemannian Hessian is hard to deal with analytically and study the suitability of different trace estimation methods~\cite{hutchinson1989stochastic,meyer2020hutch}.
We find that both vanilla Hutchinson and its variance-reduced counterpart Hutch++~\cite{meyer2020hutch} work reliably for the Euclidean case.
However, the vanilla Hutchinson trace estimator can suffer from high variance throughout an orbit of the symmetry group when applied to the Riemannian Hessian.
Variance-reduced methods like Hutch++ offer higher quality trace estimates in such cases.

\begin{figure}[tb]
  \centering
  \begin{subfigure}{1.0\linewidth}
    \caption{}\label{subfig:shallow-linear-matrix-valued-a}
    \includegraphics{../../symmetry_exp/exp05_two_layer_matrix/hutchinson_vs_hutchpp.pdf}
  \end{subfigure}
  \begin{subfigure}{1.0\linewidth}
    \caption{}\label{subfig:shallow-linear-matrix-valued-b}
    \includegraphics{../../symmetry_exp/exp05_two_layer_matrix/euclidean_vs_riemannian.pdf}
  \end{subfigure}
  \begin{subfigure}{1.0\linewidth}
    \caption{}\label{subfig:shallow-linear-matrix-valued-c}
    \includegraphics{../../symmetry_exp/exp05_two_layer_matrix/spectra.pdf}
  \end{subfigure}
  \caption{\emph{Trace estimation of the Euclidean and Riemannian Hessians on a shallow linear network with matrix-valued weights on MNIST.}
    (\subref{subfig:shallow-linear-matrix-valued-a}) Comparison between vanilla Hutchinson and Hutch++ trace estimation along a curve through an orbit $\vtheta(\alpha)$ of the symmetry group.
    Both methods reliably estimate the Euclidean Hessian's, but only Hutch++ reliably estimates the Riemannian Hessian's trace.
    Error bars correspond two standard deviations above and below the mean obtained from the samples generated with the assigned matrix-vector product budget.
    (\subref{subfig:shallow-linear-matrix-valued-b}) Relative error of the Euclidean and Riemannian Hessian's trace estimation for two different points on the curve through the orbit.
    In the Euclidean case, both estimators exhibit roughly the same approximation quality.
    In the Riemannian case, Hutch++ is significantly more accurate than vanilla Hutchinson.
    For improved visibility, all curves were smoothed with an exponential moving average.
    (\subref{subfig:shallow-linear-matrix-valued-c}) Eigenvalue spectra of the Euclidean and Riemannian Hessians at three points on the curve, re-scaled by their largest magnitude eigenvalues.
    We only show the top and bottom eigenvalues that significantly differ from zero.
    Hutchinson's trace estimate suffers from high variance for small and large values of $\alpha$.
    For those points, the Riemannian Hessian's spectrum is `less flat' compared to the Euclidean Hessian's spectrum.
  }
  \label{fig:shallow-linear-matrix-valued}
\end{figure}

\paragraph{Setup} We use a shallow linear network with matrix-valued weights $\mW^{(1)} \in \R^{h \times D_{\text{in}}}$ and $\mW^{(2)} \in \R^{D_{\text{out}} \times h}$ without bias terms.
As data, we randomly draw a single mini-batch with $N=128$ examples from the
MNIST training data set, $\sD = \left\{ (\vx_n, \vy_n) \in \sR^{D_{\text{in}}}\times \sR^{D_{\text{out}}} \mid n=1,\dots, N \right\}$ where $D_{\text{in}}=784$ and $D_{\text{out}}=10$.
We set the hidden dimension to $h=2$ such that the model exhibits a $\GL(2)$
symmetry and use softmax cross-entropy loss $\ell$ to obtain the loss
\begin{align*}
  \gL_{\sD}(\vtheta) = \frac{1}{N} \sum_{n=1}^N \ell(\mW^{(2)} \mW^{(1)} \vx_n, \vy_n)\,,
  \qquad
  \text{with}
  \qquad
  \vtheta
  =
  \begin{pmatrix}
    \flatten \mW^{(1)}
    \\
    \flatten \mW^{(2)}
  \end{pmatrix}
  \in \sR^{h (D_{\text{out}} + D_{\text{in}})}\,,
\end{align*}
where $\flatten$ denotes column-stacking and $D \coloneqq h (D_{\text{out}} + D_{\text{in}})$ is the total number of parameters.

We investigate the trace of the Euclidean Hessian
\begin{align*}
  \operatorname{Hess}_\text{E} \gL_{\sD}(\vtheta)
  \coloneqq
  \frac{\partial^2 \gL_{\sD}(\vtheta)}{\partial \vtheta \partial \vtheta^\top}
  \in \sR^{D \times D}
\end{align*}
and the Riemannian Hessian $\operatorname{Hess}_\text{R} \gL_{\sD}(\vtheta): \sR^D \to \sR^D$, defined by a correction to the Euclidean Hessian via \Cref{equ:riemannian-hessian-corrections}.

\paragraph{Curve through orbit} We consider the trace's behavior along a smooth curve $\vtheta(\alpha): \sR \to \sR^D, \alpha \mapsto \vtheta(\alpha)$ in parameter space that remains in a fixed orbit.
Starting with the randomly initialized network weights $\mW^{(1)}_0,
\mW^{(2)}_0$, we draw a random matrix $\mA \in \GL(h)$ with uniformly
distributed eigenvalues over $[-10; -1] \cup [1; 10]$. We then use $\alpha \mA$
to parameterize the curve via
\begin{align*}
  \begin{pmatrix}
    \mW^{(1)}
    \\
    \mW^{(2)}
  \end{pmatrix}
  (\alpha)
  =
  \begin{pmatrix}
    \left( \alpha \mA \right) \mW^{(1)}_0
    \\
    \mW^{(2)}_0 \left( \alpha \mA \right)^{-1}
  \end{pmatrix}
  \qquad
  \Leftrightarrow
  \qquad
  \vtheta(\alpha)
  =
  \begin{pmatrix}
    \flatten \left(
    \alpha \mA \mW^{(1)}_0
    \right)
    \\
    \flatten \left(
    \alpha^{-1} \mW^{(2)}_0 \mA^{-1}
    \right)
  \end{pmatrix}\,.
\end{align*}
All points on the curve through the orbit have the same empirical risk.

\paragraph{Trace estimation} As $D$ is relatively small in this experiment, we can evaluate the exact traces by computing matrix-vector products with the unit vectors and use them as ground truth.
In practise though, both $D$ and computational work to perform a matrix-vector products may be large.
Hence, we use stochastic trace estimation methods that require less than $D$ matrix-vector products and study their approximation quality.
Specifically, we use vanilla Hutchinson trace estimation and Hutch++, a variance-reduced version of the former.
For vanilla Hutchinson, drawing a sample from the trace estimator involves a single matrix-vector product with a randomly generated query vector (we use Rademacher).
Hutch++ is similar in that drawing a new sample involves a single matrix-vector product.
Initializing the estimator involves an initial cost for computing and evaluating the trace in a low-dimensional basis $\mQ \in \sR^{D \times k}$ with $2k$ matrix-vector products (we use $k=20$).
For a fair comparison between both methods, we allow the same computational budget of 100 matrix-vector products.

\paragraph{Metrics} Let $T \in \sR$ be a placeholder for the exact trace of either the Euclidean or Riemannian Hessian and let $\hat{T} \in \sR$ denote a sample from one of the investigated trace estimators.
As the Hessian's trace can be negative, we show its absolute value $|T|$ or $|\hat{T}|$ in \Cref{subfig:shallow-linear-matrix-valued-a}.
Error bars span two standard deviations above and below the mean and were obtained from the samples generated with the assigned matrix-vector product budget.
To compare the approximation quality for different points on the curve through
the orbit, we use the relative error $\nicefrac{|T - \hat{T} |}{|T|}$ (see for
instance \Cref{subfig:shallow-linear-matrix-valued-b}).

\paragraph{Results} Figure \Cref{subfig:shallow-linear-matrix-valued-a} shows the Euclidean and Riemannian Hessian traces throughout the curve through an orbit and compares vanilla Hutchinson with Hutch++.
As expected, the Riemannian Hessian's trace is constant, while the Euclidean Hessian's trace varies significantly.
Both Hutchinson and Hutch++ work reliably for the Euclidean Hessian, but Hutch++ works more reliably for the Riemannian Hessian, showing significantly smaller confidence intervals (right panel).

Figure \Cref{subfig:shallow-linear-matrix-valued-b} complements this view from a different angle.
It shows the relative error's evolution w.r.t.\,the invested number of matrix-vector multiplies for two different points on the curve through the orbit.
In the Euclidean case (left panel), the approximation quality of both trace estimation methods follows the same trend.
But in the Riemannian case (right panel), Hutch++'s approximation error is more than two orders of magnitude lower after 100 matrix-vector products.

Hutchinson's trace estimation works well for matrices with a flat spectrum.
Our findings that Hutchinson fails to accurately estimate the trace for the Riemannian case suggests that the Riemannian corrections render the spectrum less flat and therefore the trace more challenging to estimate.
\Cref{subfig:shallow-linear-matrix-valued-b} compares the Euclidean and Riemannian Hessian's spectra for three points along the curve through the orbit.
For very small or very large values of $\alpha$, the Riemannian Hessian's spectrum indeed seems to be `less flat' than the Euclidean Hessian's spectrum.

%%% Local Variables:
%%% mode: latex
%%% TeX-master: "../main"
%%% End:
