# Supplementary material for: Hide & Seek: Transformer Symmetries Obscure Sharpness & Riemannian Geometry Finds It
Source: arXiv:2505.05409 source file (2025-05-08)
Supplement: Supplementary file 3 [file shallow_linear_net_scalar_weights.tex]

Here we apply the results from the main text to a small toy example that was used to generate \Cref{fig:visualization-scalar-toy}.

\paragraph{Model} Consider a shallow linear network from \Cref{ex:shallow-linear-net} with one-dimensional input and output domain such that both weights are scalars.
I.e.
$\vtheta = \smash{\begin{pmatrix} \theta_1 & \theta_2 \end{pmatrix}^{\top}} \in \sR^2$ and $f_{\vtheta}: \sR \times \sR^2 \to \sR, (\vtheta, x) \mapsto f_{\vtheta}(x) = \theta_2 \theta_1 x$.
The neural network multiplies its input with a single number $\theta_2 \theta_1$.
Hence, its effective dimensionality is one, while the parameter space is two-dimensional.
When comparing to the canonical form, we can make the following identifications:
\begin{itemize}
\item Parameters:
  \begin{align*}
    (\mG, \mG^\top) \leftrightarrow \theta_2
    \qquad
    \text{and}
    \qquad
    (\mH, \mH^\top) \leftrightarrow \theta_1
  \end{align*}

\item Tangent vector components:
  \begin{align*}
    \xi
    =
    \begin{pmatrix}
      \xi_{\mG} \\ \xi_{\mH}
    \end{pmatrix}
    \leftrightarrow
    \xi =
    \begin{pmatrix}
      \xi_{\theta_2} \\ \xi_{\theta_1}
    \end{pmatrix}
  \end{align*}

\item Euclidean gradient components:
  \begin{align*}
    \partial f
    =
    \begin{pmatrix}
      \partial_{\mG} \ell \\ \partial_{\mH} \ell
    \end{pmatrix}
    \leftrightarrow
    \partial f
    =
    \begin{pmatrix}
      \partial_{\theta_2} \ell \\ \partial_{\theta_1} \ell
    \end{pmatrix}
  \end{align*}

\item Euclidean Hessian components:
  \begin{align*}
    \partial^2 \ell
    =
    \begin{pmatrix}
      \partial^2_{\mG,\mG} \ell & \partial^2_{\mG,\mH} \ell \\
      \\
      \partial^2_{\mH,\mG} \ell & \partial^2_{\mH,\mH} \ell
    \end{pmatrix}
    =
    \begin{pmatrix}
      \partial^2_{\mG,:} \ell \\ \partial^2_{\mH,:} \ell
    \end{pmatrix}
    \leftrightarrow
    \partial^2 \ell
    =
    \begin{pmatrix}
      \partial^2_{\theta_2,\theta_2} \ell & \partial^2_{\theta_2,\theta_1} \ell
      \\
      \partial^2_{\theta_1,\theta_2} \ell & \partial^2_{\theta_1,\theta_1} \ell
    \end{pmatrix}
    =
    \begin{pmatrix}
      \partial^2_{\theta_2,:} \ell \\ \partial^2_{\theta_1,:} \ell
    \end{pmatrix}
  \end{align*}
\item Riemannian gradient components
  \begin{align*}
    \tilde{\partial} \ell
    =
    \begin{pmatrix}
      \tilde{\partial}_{\mG} \ell \\ \tilde{\partial}_{\mH} \ell
    \end{pmatrix}
    \leftrightarrow
    \tilde{\partial} \ell
    =
    \begin{pmatrix}
      \tilde{\partial}_{\theta_2} \ell \\ \tilde{\partial}_{\theta_1} \ell
    \end{pmatrix}
  \end{align*}
\item Riemannian Hessian components before lifting
  \begin{align*}
    \tilde{\partial}^2 \ell
    =
    \begin{pmatrix}
      \tilde{\partial}^2_{\mG,\mG} \ell & \tilde{\partial}^2_{\mG,\mH} \ell \\
      \\
      \tilde{\partial}^2_{\mH,\mG} \ell & \tilde{\partial}^2_{\mH,\mH} \ell
    \end{pmatrix}
    =
    \begin{pmatrix}
      {\tilde{\partial}^2_{\mG,:} \ell}^{\mathcal{H}} \\ \tilde{\partial}^2_{\mH,:} \ell
    \end{pmatrix}
    \leftrightarrow
    \tilde{\partial}^2 \ell
    =
    \begin{pmatrix}
      \tilde{\partial}^2_{\theta_2,\theta_2} \ell & \tilde{\partial}^2_{\theta_2,\theta_1} \ell
      \\
      \tilde{\partial}^2_{\theta_1,\theta_2} \ell & \tilde{\partial}^2_{\theta_1,\theta_1} \ell
    \end{pmatrix}
    =
    \begin{pmatrix}
      \tilde{\partial}^2_{\theta_2,:} \ell \\ \tilde{\partial}^2_{\theta_1,:} \ell
    \end{pmatrix}
  \end{align*}
\end{itemize}

\paragraph{Data} We generate a synthetic regression data set $\sD = \left\{ (x_n, y_n) \in \sR \times \sR \mid n=1, \dots, N \right\}$ with $N = TODO$ samples generated from the relation $y_n = TODO x_n + \epsilon_n$ where $\epsilon_n \sim TODO$.

\paragraph{Loss function} The network's output is scored with square loss, so the empirical risk, shown in the top left panel of \Cref{fig:visualization-scalar-toy}, is
\begin{subequations}
  \begin{align}
    \gL_{\sD}(\vtheta)
    &=
      \frac{1}{N} \sum_{n=1}^N \left( f_{\vtheta}(x_n) - y_n \right)^2
      =
      \frac{1}{N} \sum_{n=1}^N
      \underbrace{
      \left( \theta_2 \theta_1 x_n - y_n \right)^2
      }_{\coloneqq \ell_n(\vtheta)}\,.
      \shortintertext{To remove unnecessary clutter from the derivations, we focus on a per-datum loss}
      \ell(\vtheta) &= \left( f_{\vtheta}(x) - y \right)^2
                      = \left( \theta_2 \theta_1 x - y \right)^2\,.
  \end{align}
\end{subequations}
We can introduce the averages over all data points post-hoc without loss of generality.

\subsection{Euclidean quantities}

\paragraph{Euclidean metric} The Euclidean metric is equivalent to the dot product:
\begin{align}
  g(\xi, \eta)
  =
  \xi_{\theta_2} \eta_{\theta_2} + \xi_{\theta_1} \eta_{\theta_1}\,.
\end{align}

\paragraph{Euclidean gradient} The Euclidean gradient is the vector containing the loss's first partial derivatives:
\begin{align}
  \partial \ell
  =
  \begin{pmatrix}
    \partial_{\theta_2} \ell
    \\
    \partial_{\theta_1} \ell
  \end{pmatrix}
  =
  \begin{pmatrix}
    \dfrac{\partial \ell}{\partial \theta_2}
    \\
    \dfrac{\partial \ell}{\partial \theta_1}
  \end{pmatrix}
  =
  2x \left( \theta_2 \theta_1 x - y \right)
  \begin{pmatrix}
    \theta_1 \\ \theta_2
  \end{pmatrix}\,.
\end{align}

\paragraph{Euclidean gradient norm} The squared Euclidean gradient norm is
\begin{align}
  g(\partial \ell, \partial \ell)
  =
  \left(
  \partial_{\theta_2} \ell
  \right)^2
  +
  \left(
  \partial_{\theta_1} \ell
  \right)^2
  =
  \left[ 2x \left( \theta_2\theta_1 x - y \right)  \right]^2
  \left(
  \theta_1^2 + \theta_2^2
  \right)\,.
\end{align}
Note that it does not exhibit $\GL$ symmetry.

\paragraph{Euclidean Hessian} The Euclidean Hessian is a matrix containing the second partial derivatives of the loss:
\begin{align}
  \partial^2 \ell
  =
  \begin{pmatrix}
    \partial^2_{\theta_2,:} \ell
    \\
    \partial^2_{\theta_1,:} \ell
  \end{pmatrix}
  =
  \begin{pmatrix}
    \partial^2_{\theta_2,\theta_2} \ell & \partial^2_{\theta_2,\theta_1} \ell
    \\
    \partial^2_{\theta_1,\theta_2} \ell & \partial^2_{\theta_1,\theta_1} \ell
  \end{pmatrix}
  =
  \begin{pmatrix}
    \frac{\partial^2 \ell}{\partial \theta_2^2}
    &
      \frac{\partial^2 \ell}{\partial \theta_2 \partial \theta_1}
    \\
    \frac{\partial^2 \ell}{\partial \theta_1 \partial \theta_2}
    &
      \frac{\partial^2 \ell}{\partial \theta_1^2}
  \end{pmatrix}
  =
  2x
  \begin{pmatrix}
    x \theta_1^2
    &
      2 x \theta_1 \theta_2 - y
    \\
    2 x \theta_1 \theta_2 - y
    &
      x \theta_2^2
  \end{pmatrix}\,.
\end{align}
Its off-diagonal elements are symmetric under $\GL$.
The diagonal elements are not.

\paragraph{Euclidean Hessian's trace} The Euclidean Hessian's trace has circular symmetry:
\begin{align}
  \Tr(\partial^2 \ell)
  =
  2x^2
  \left(
  \theta_1^2 + \theta_2^2
  \right)\,.
\end{align}

\subsection{Riemannian quantities}

\paragraph{Riemannian metric} The Riemannian metric is a weighted dot product
\begin{align}
  \tilde{g}(\xi, \eta)
  =
  \dfrac{\xi_{\theta_2} \eta_{\theta_2}}{\theta_2^2}
  +
  \dfrac{\xi_{\theta_1} \eta_{\theta_1}}{\theta_1^2}\,.
\end{align}

\paragraph{Horizontal lift} Given a tangent vector $\xi$, we first need to solve
the following Lyapunov equation,
\begin{align*}
  \lambda \theta_2^2 \theta_1^2
  +
  \theta_2^2 \theta_1^2 \lambda
  =
  \theta_2^2 \theta_1 \xi_{\theta_1} - \xi_{\theta_2} \theta_2 \theta_1^2\,,
\end{align*}
whose solution is $\lambda = \frac{\xi_{\theta_1}}{2 \theta_1} +
\frac{\xi_{\theta_2}}{2\theta_2}$. We can then horizontally lift the tangent
vector by forming
\begin{align}
  \xi^{\mathcal{H}}
  =
  \begin{pmatrix}
    \xi^{\mathcal{H}}_{\theta_2}
    \\
    \xi^{\mathcal{H}}_{\theta_1}
  \end{pmatrix}
  =
  \begin{pmatrix}
    \xi_{\theta_2} + \theta_2 \lambda
    \\
    \xi_{\theta_1} + \theta_1 \lambda
  \end{pmatrix}
  =
  \dfrac{1}{2}
  \begin{pmatrix}
    \xi_{\theta_2} + \dfrac{\theta_2}{\theta_1} \xi_{\theta_1}
    \\
    \xi_{\theta_1} + \dfrac{\theta_1}{\theta_2} \xi_{\theta_2}
  \end{pmatrix}\,.
\end{align}
This can also be written as matrix-vector multiplication with the projector $\Pi^{\mathcal{H}}$,
\begin{align}
  \xi^{\mathcal{H}} = \Pi^{\mathcal{H}} \xi
  \qquad
  \text{where}
  \qquad
  \Pi^{\mathcal{H}}
  =
  \dfrac{1}{2}
  \begin{pmatrix}
    1 & \dfrac{\theta_2}{\theta_1}
    \\
    \dfrac{\theta_1}{\theta_2} & 1
  \end{pmatrix}\,.
\end{align}
We can convince ourselves that, indeed, this is a projector, as it satisfies the
idempotence property $\Pi^{\mathcal{H}}\Pi^{\mathcal{H}} = \Pi^{\mathcal{H}}$:
\begin{align}
  \Pi^{\mathcal{H}}\Pi^{\mathcal{H}}
  =
  \dfrac{1}{2}
  \begin{pmatrix}
    1 & \dfrac{\theta_2}{\theta_1}
    \\
    \dfrac{\theta_1}{\theta_2} & 1
  \end{pmatrix}
  \dfrac{1}{2}
  \begin{pmatrix}
    1 & \dfrac{\theta_2}{\theta_1}
    \\
    \dfrac{\theta_1}{\theta_2} & 1
  \end{pmatrix}
  =
  \dfrac{1}{4}
  \begin{pmatrix}
    2 & 2\dfrac{\theta_2}{\theta_1}
    \\
    2\dfrac{\theta_1}{\theta_2} & 2
  \end{pmatrix}
  =
  \dfrac{1}{2}
  \begin{pmatrix}
    1 & \dfrac{\theta_2}{\theta_1}
    \\
    \dfrac{\theta_1}{\theta_2} & 1
  \end{pmatrix}
  =
  \Pi^{\mathcal{H}}\,.
\end{align}

\paragraph{Riemannian gradient} The Riemannian gradient follows from the
Euclidean gradient as
\begin{align}
  \begin{split}
    \tilde{\partial}\ell
    =
    \begin{pmatrix}
      \tilde{\partial}_{\theta_2}\ell
      \\
      \tilde{\partial}_{\theta_1}\ell
    \end{pmatrix}
    &=
      \begin{pmatrix}
        (\partial_{\theta_2}\ell) \theta_2^2
        \\
        (\partial_{\theta_1}\ell) \theta_1^2
      \end{pmatrix}
    \\
    &\text{(insert Euclidean gradient)}
    \\
    &=
      2 x \left( \theta_2 \theta_1 x - y \right)
      \begin{pmatrix}
        \theta_1 \theta_2^2
        \\
        \theta_2 \theta_1^2
      \end{pmatrix}\,.
  \end{split}
\end{align}

\paragraph{Riemannian gradient norm} The squared Riemannian gradient's norm has $\GL$ symmetry:
\begin{align}
  \begin{split}
    \tilde{g}(\tilde{\partial}\ell, \tilde{\partial}\ell)
    &=
      \dfrac{(\tilde{\partial}_{\theta_2}\ell)^2}{\theta_2^2}
      +
      \dfrac{(\tilde{\partial}_{\theta_1}\ell)^2}{\theta_1^2}
    \\
    &\text{(express via Euclidean gradient)}
    \\
    &=
      \theta_2^2 (\partial_{\theta_2}\ell)^2
      +
      \theta_1^2 (\partial_{\theta_1}\ell)^2
    \\
    &\text{(insert Euclidean gradient, simplify)}
    \\
    &=
      2 \left[ 2x \left( \theta_2 \theta_1 x - y \right) \right]^2
      \left( \theta_2 \theta_1 \right)^2
  \end{split}
\end{align}

\paragraph{Riemannian Hessian} Let's take this part slowly, because the expressions in the main text are not there yet.
The Riemannian Hessian's lift ${\tilde{\partial}^{2}\ell}^{\mathcal{H}}$ acts on a tangent vector $\xi$ as follows: $\xi \mapsto \Pi^{\mathcal{H}} ((\tilde{\partial}^2\ell) \xi)$.
Here, $\tilde{\partial}^2\ell$ is the Riemannian Hessian before lifting.
Our strategy will be as follows: First, we will compute the matrix representation of the Riemannian Hessian before lifting, following the derivations from the ManOpt library (\href{https://www.manopt.org/manifold_documentation_fixedrank_2factors.html}{here}).
Then, we can simply multiply the projection operator from the left to obtain a matrix representation of the Riemannian Hessian, such that its action on a tangent vector is $(\tilde{\partial}^2\ell^{\mathcal{H}}) \xi = (\Pi^{\mathcal{H}} \tilde{\partial}^2\ell) \xi$.

We can start from the ManOpt documentation to obtain the Riemannian Hessian
before lifting. Specifically, we have
\begin{align*}
  (\tilde{\partial}^2\ell) \xi
  =
  \begin{pmatrix}
    (\tilde{\partial}_{\mG,:}^2\ell) \xi
    \\
    (\tilde{\partial}_{\mH,:}^2\ell) \xi
  \end{pmatrix}
\end{align*}
where each of the components is a corrected Hessian-vector product,
\begin{align*}
  \begin{split}
    (\tilde{\partial}_{\mG,:}^2\ell) \xi
    &=
      ((\partial^2_{\mG}\ell)  \xi) \mG^{\top} \mG
    \\
    &+ 2 (\partial_{\mG}\ell) \sym \left(\mG^{\top} \xi_{\mG}\right)
    \\
    &- \xi_{\mG} \left( \mG^{\top}\mG \right)^{-1} \sym \left( \mG^{\top} \tilde{\partial}_{\mG}\ell \right)
    \\
    &- \partial_{\mG}\ell \sym \left( \mG^{\top}\xi_{\mG} \right)
    \\
    &+ \mG \left( \mG^{\top} \mG \right)^{-1} \sym \left( \xi_{\mG}^{\top} \tilde{\partial}_{\mG}\ell\right)
  \end{split}
  \intertext{and}
  \begin{split}
    (\tilde{\partial}_{\mH,:}^2\ell) \xi
    &=
      ((\partial^2_{\mH}\ell)  \xi) \mH^{\top} \mH
    \\
    &+ 2 (\partial_{\mH}\ell) \sym \left(\mH^{\top} \xi_{\mH}\right)
    \\
    &- \xi_{\mH} \left( \mH^{\top}\mH \right)^{-1} \sym \left( \mH^{\top} \tilde{\partial}_{\mH}\ell \right)
    \\
    &- \partial_{\mH}\ell \sym \left( \mH^{\top}\xi_{\mH} \right)
    \\
    &+ \mH \left( \mH^{\top} \mH \right)^{-1} \sym \left( \xi_{\mH}^{\top} \tilde{\partial}_{\mH}\ell\right)\,.
  \end{split}
\end{align*}
For our scalar problem, we have the simplification that $a, b \in \sR \implies
\sym(ab) = ab$. Also, taking the inverse becomes taking the reciprocal.

Let's compute the action of $\tilde{\partial}_{\theta_2,:}^2\ell$ onto $\xi$:
\begin{align*}
  \begin{split}
    (\tilde{\partial}_{\theta_2,:}^2\ell) \xi
    =
    (\tilde{\partial}_{\theta_2, \theta_2}) \xi_{\theta_2}
    +
    (\tilde{\partial}_{\theta_2, \theta_1}) \xi_{\theta_1}
    &=
      ((\partial^2_{\theta_2}\ell)  \xi) \theta_2^2
    \\
    &+ 2 (\partial_{\theta_2,:}\ell) \theta_2 \xi_{\theta_2}
    \\
    &- \xi_{\theta_2} \dfrac{1}{\theta_2^2} \theta_2 \tilde{\partial}_{\theta_2}\ell
    \\
    &- \partial_{\theta_2}\ell \theta_2\xi_{\theta_2}
    \\
    &+ \theta_2 \dfrac{1}{\theta_2^2} \xi_{\theta_2} \tilde{\partial}_{\theta_2}\ell
    \\
    &\text{(insert Riemannian gradient)}
    \\
    &=
      ((\partial^2_{\theta_2,:}\ell)  \xi) \theta_2^2
    \\
    &+ 2 (\partial_{\theta_2}\ell) \theta_2 \xi_{\theta_2}
    \\
    &- \xi_{\theta_2} \dfrac{1}{\theta_2^2} \theta_2 \partial_{\theta_2}\ell \theta_2^2
    \\
    &- \partial_{\theta_2}\ell \theta_2\xi_{\theta_2}
    \\
    &+ \theta_2 \dfrac{1}{\theta_2^2} \xi_{\theta_2} \partial_{\theta_2}\ell \theta_2^2
    \\
    &\text{(simplify)}
    \\
    &=((\partial^2_{\theta_2,:}\ell)  \xi) \theta_2^2
      +
      \theta_2 \xi_{\theta_2} \partial_{\theta_2}\ell
    \\
    &\text{(insert Euclidean Hessian blocks)}
    \\
    &= \left[ (\partial^2_{\theta_2, \theta_2}\ell) \xi_{\theta_2} + (\partial^2_{\theta_2, \theta_1}\ell) \xi_{\theta_1} \right] \theta_2^2
      + \theta_2 \xi_{\theta_2} \partial_{\theta_2}\ell
    \\
    &\text{(insert Euclidean Hessian and Euclidean gradient)}
    \\
    &=
      \left[
      \left( 2x^2 \theta_1^2 \right) \xi_{\theta_2}
      +
      2\left( 2x \theta_1\theta_2 - y  \right) \xi_{\theta_1}
      \right] \theta_2^2
      +
      2x \theta_2\theta_1\left( \theta_2 \theta_1x - y \right) \xi_{\theta_2}
    \\
    &\text{(simplify and group by components of $\xi$ to identify the matrix components)}
    \\
    &=
      \underbrace{
      \left[
      2 \theta_1\theta_2 x \left( 2 \theta_2\theta_1 x - y \right)
      \right]
      }_{\tilde{\partial}^2_{\theta_2, \theta_2}\ell}
      \xi_{\theta_2}
      +
      \underbrace{
      \left[
      2 \theta_2^2 x \left( 2 \theta_2\theta_1x - y \right)
      \right]
      }_{\tilde{\partial}^2_{\theta_2, \theta_1}\ell}
      \xi_{\theta_1}
  \end{split}
\end{align*}
The action of $\tilde{\partial}_{\theta_1,:}^2\ell$ onto $\xi$ is analogous, but
exchanges the role of $\theta_1$ and $\theta_2$. Hence we obtain the two other components
\begin{align*}
  \begin{split}
    \tilde{\partial}^2_{\theta_1, \theta_2}\ell
    &=
      2 \theta_1^2x \left( 2 \theta_2\theta_1 x - y \right)
    \\
    \tilde{\partial}^2_{\theta_1, \theta_1}\ell
    &=
      2 \theta_1\theta_2 x \left( 2 \theta_2\theta_1 x - y \right)\,.
  \end{split}
\end{align*}
We can now write down the action $(\tilde{\partial}^2\ell)\xi$ as matrix-vector product:
\begin{align*}
  (\tilde{\partial}\ell^2)\xi
  =
  2x \left( 2\theta_1 \theta_2 x - y \right)
  \begin{pmatrix}
    \theta_1\theta_2 & \theta_2^2
    \\
    \theta_1^2 & \theta_1\theta_2
  \end{pmatrix}
  \begin{pmatrix}
    \xi_{\theta_2}
    \\
    \xi_{\theta_1}
  \end{pmatrix}
\end{align*}
Note that, \textbf{strangely}, the matrix multiplied onto $\xi$ is not symmetric.
Let's accept that for now, because we still haven't done the lifting part yet.
After multiplying with the projector for the horizontal lift, we obtain
\begin{align*}
  \begin{split}
    {\tilde{\partial}^2\ell}^{\mathcal{H}} \xi
    =
    \Pi^{\mathcal{H}} \tilde{\partial}^2\ell \xi
    &=
      \dfrac{1}{2}
      \begin{pmatrix}
        1 & \dfrac{\theta_2}{\theta_1}
        \\
        \dfrac{\theta_1}{\theta_2} & 1
      \end{pmatrix}
      2x \left( 2\theta_1 \theta_2 x - y \right)
      \begin{pmatrix}
        \theta_1\theta_2 & \theta_2^2
        \\
        \theta_1^2 & \theta_1\theta_2
      \end{pmatrix}
      \xi
    \\
    &=
      \underbrace{
      2x \left( 2\theta_1\theta_2 x - y \right)
      \begin{pmatrix}
        \theta_1 \theta_2 & \theta_2^2
        \\
        \theta_2^2 & \theta_1 \theta_2
      \end{pmatrix}
      }_{{\tilde{\partial}^2\ell}^{\mathcal{H}}}
      \xi\,.
  \end{split}
\end{align*}
Note that, \textbf{still}, this matrix is not symmetric.

\paragraph{Riemannian Hessian trace} The problem from above is still unresolved.
But it does not seem to affect the trace's $\GL$ symmetry,
\begin{align*}
  \Tr \left( {\tilde{\partial}^2\ell}^{\mathcal{H}} \right)
  =
  4x \left( \theta_1 \theta_2x -y \right) \theta_1 \theta_2\,.
\end{align*}

%%% Local Variables:
%%% mode: latex
%%% TeX-master: "../main"
%%% End:
