# Supplementary material for: Hide & Seek: Transformer Symmetries Obscure Sharpness & Riemannian Geometry Finds It
Source: arXiv:2505.05409 source file (2025-05-08)
Supplement: Supplementary file 4 [file variance_reduced_hutchinson.tex]

\section{[FAIL] Variance-reduced Hutchinson's trace estimator}

\subsection{Method}
Consider a linear operator \(\mA \in \sR^{D \times D}\). Hutchinson's trace
estimator is given by
\begin{align}
  \hat{Z} := \vx^{\top} \mA \vx\,, \quad \vx \sim \gN(\vzero, \mI)\,.
\end{align}
We can reduce the variance of \(\hat{Z}\) by introducing a control variate \(\mB
\in \sR^{D \times D}\) (which is somehow easier to deal with than \(\mA\)) and
using the estimator
\begin{align}
  \hat{Z}'
  :=
  \vx^{\top} \mA \vx
  -
  c \left( \vx^{\top} \mB \vx - \Tr(\mB) \right)\,,
  \qquad
  \vx \sim \gN(\vzero, \mI)\,, c \in \sR\,.
\end{align}
Both are unbiased estimators of the trace, \(\E\left[ \hat{Z} \right] = \E\left[
  \hat{Z}' \right] = \Tr\left( \mA \right)\). Lemma 4.1 of
\cite{adams2018estimating} states provides the optimal value of \(c_{\star}\)
that minimizes the variance of \(\hat{Z}'\) as
\begin{align}
  c_{\star}
  =
  \frac{
  \Tr \left( \mA \mB \right)
  }{
  \Tr \left( \mB^{\top} \mB \right)
  }\,.
\end{align}
For any \(c\), the variance reduction is
\begin{align}
  \Var \left[ \hat{Z} \right]
  -
  \Var \left[ \hat{Z}' \right]
  =
  4c \Tr \left( \mA \mB \right)
  -
  2c^2 \Tr \left( \mB^{\top} \mB \right)\,.
\end{align}
The maximum variance reduction, achieved by setting \(c \gets c_{\star}\), is
\begin{align}
  2 \frac{
  \left[ \Tr \left( \mA \mB \right) \right]^2
  }{
  \Tr \left( \mB^{\top} \mB \right)
  }\,.
\end{align}
The regular Hutchinson trace estimator has variance \(\Var \left[ \hat{Z}
\right] = 2 \Tr \left( \mA^{\top} \mA \right) = 2 \left\lVert \mA
\right\rVert^2_{\text{F}}\). Hence, the relative optimal variance reduction is
\begin{align}
  1
  -
  \frac{
  \Var \left[ \hat{Z} \right] - \Var \left[ \hat{Z}' \right]
  }{
  \Var \left[ \hat{Z} \right]
  }
  \overset{(c = c_{\star})}{=}
  1
  -
  \frac{
  \left[ \Tr \left( \mA\mB^{\top} \right) \right]^2
  }{
  \Tr \left( \mB \mB^{\top} \right)
  \Tr \left( \mA \mA^{\top} \right)
  }\,.
\end{align}

\paragraph{Using known matrix-vector products as control variate:} Assume we
know the matrix-vector products \(\vv_k^{\top} \mA \vv_k\) for \(k = 1, \dots,
K\). We can incorporate this knowledge into the trace estimation via a control
variate by setting \(\mB := \mV \mV^{\top}\) with \(\mV = (\vv_1, \dots, \vv_K)
\in \sR^{D \times K}\). The Hutchinson trace estimator with control variate
becomes
\begin{align}
  \hat{Z}'
  =
  \vx^{\top} \mA \vx
  -
  c \left(
  \sum_{k=1}^K
  \left( \vv_k^{\top} \vx \right)^2
  -
  \left\lVert \vv_k \right\rVert_2^2
  \right)\,.
\end{align}
(The second term in the parentheses only needs to be computed once.) The optimal
value for \(c\) that minimizes \(\Var \left[ \hat{Z}' \right]\) is
\begin{align}
  c_{\star}
  =
  \frac{
  \sum_{k=1}^K \vv_k^{\top} \mA \vv_k
  }{
  \Tr \left( \mV^{\top} \mV \mV^{\top} \mV \right)
  }\,.
\end{align}
It \textbf{incorporates the known matrix-vector products} and only needs to be
computed once.

\paragraph{Note:} Using vectors with known matrix-vector product may not
significantly reduce the variance if the vectors don't overlap with directions
of large eigenvalues. Hence, incorporating this knowledge may not save
computations, even add additional ones because we need to compute the \(K\) dot
products with \(\vx\). A better objective for choosing control variate vectors
are vectors that overlap with large eigenvalues, for instance as done in
\cite{meyer2020hutch}.

\subsection{Estimating the Hessian Trace in the Presence of Scaling Symmetry}
\paragraph{Motivation:} In \cite{kunin2021symmetry}, scaling symmetry imposes a
relation between the Hessian, the loss gradient, and the parameters,
\Cref{eq:scaling-constraints}. This relation is exact in the limit of
infinitesimally small parameter updates (learning rate $\rightarrow 0$), but
since models aren't trained in that regime the possibility exists that real-life
models do violate the restrictions imposed by symmetry.

\paragraph{Experiment:} In this experiment, we take a small model that contains
the sequence $\text{Conv2d} \rightarrow \text{BatchNorm2d}$. The loss is
invariant under scaling the convolution's parameters and the relation $H\theta +
g = 0$ is expected to hold. We verify this constraint holds in this experiment.
Also, if the Hessian were invertible, we could get a Newton step by rearranging
to $- H^{-1} g = \theta$. In this experiment, we probe whether both ways of
computing the Newton step (LHS vs. RHS) match.

\paragraph{Results:} As it turns out, the Hessian is close to singular, which
spoils the constraint for the Hessian inverse. Nevertheless, we still show that
(i) the constraint holds in the subspace spanned by the Hessian's nontrivial
eigenvectors, and (ii) motivate that looking at the parameters instead of
computing the Newton step with inverse HVPs is much cheaper.

%%% Local Variables:
%%% mode: latex
%%% TeX-master: "../main"
%%% End:
