# Supplementary material for: Hide & Seek: Transformer Symmetries Obscure Sharpness & Riemannian Geometry Finds It
Source: arXiv:2505.05409 source file (2025-05-08)
Supplement: Supplementary file 5 [file additional_analysis_kunin.tex]

The Hessian is often approximated through other quantities, such as the
GGN/Fisher or the empirical Fisher and we want to better understand whether
these proxies are constrained in the same way as the Hessian, or differently.

\fd{We could also look at other objects that people care about, like the
  empirical NTK.}

\subsubsection{Model Jacobian}
\label{sec:model-jacobian}
Approximations of the Hessian almost always use the model's Jacobian. Let $f:
\sR^D \times \sR^C: \vtheta \mapsto f(\vtheta)$ denote the neural network's
$C$-dimensional output. We can imagine $f$ to consist of components $f_1, \dots,
f_C$. If $f$ is invariant under an action $\psi$ of a continuous group, then the
same constraints as in \Cref{sec:background} hold, but \emph{for each component
  of $f$}. We will now translate the gradient constraints and express them in
terms of the model's Jacobian $\left.\mJ f \right\rvert_{\vtheta} =
(\left.\nabla f_1 \right\rvert_{\vtheta}, \dots, \left.\nabla f_C
\right\rvert_{\vtheta}) \in \sR^{C \times D}$.

\paragraph{Translation symmetry:} \fd{TODO}

\paragraph{Scale symmetry:} \fd{TODO}

\paragraph{Re-scale symmetry:} \fd{TODO}

\subsubsection{Popular curvature approximations}
Here, we define the Hessian, GGN, and empirical Fisher on a data set (or mini-batch).
\begin{align}
  \mH = \text{\fd{(TODO Define Hessian)}}
  \\
  \mG = \text{\fd{(TODO Define GGN/Fisher)}}
  \\
  \mK = \text{\fd{(TODO Define empirical Fisher)}}
\end{align}
Based on the model Jacobian's constraints from \Cref{sec:model-jacobian}, we can
make the following connections between $\mH$ and its common approximations $\mG,
\mK$:
\begin{itemize}
\item Translation symmetry
  \begin{align*}
    \mG \vone_{\sA} = \mK \vone_{\sA} = \mH \vone_{\sA} = \vzero
  \end{align*}

\item Scale symmetry

\item Re-scale symmetry
\end{itemize}

%%% Local Variables:
%%% mode: latex
%%% TeX-master: "../main"
%%% End:
